# Supplementary material for: Tunable Room Temperature Magnetic Skyrmions in Ir/Fe/Co/Pt Multilayers
Source: arXiv:1606.06034 ancillary file (2017-07-17)
Supplement: Supplementary file 1 [file SkTuning_SM.pdf]

# Supplementary Information for

## Tunable Room Temperature Magnetic Skyrmions in Ir/Fe/Co/Pt Multilayers

Anjan Soumyanarayanan,<sup>1,2,\*</sup> M. Raju,<sup>2</sup> A. L. Gonzalez Oyarce,<sup>1</sup> Anthony K. C. Tan,<sup>2</sup> Mi-Young Im,<sup>3,4</sup>  
A. P. Petrović,<sup>2</sup> Pin Ho,<sup>1</sup> K. H. Khoo,<sup>5</sup> M. Tran,<sup>1</sup> C. K. Gan,<sup>5</sup> F. Ernult,<sup>1</sup> and C. Panagopoulos<sup>2,†</sup>

<sup>1</sup>Data Storage Institute, 2 Fusionopolis Way, 138634 Singapore

<sup>2</sup>Division of Physics and Applied Physics, School of Physical and Mathematical Sciences,  
Nanyang Technological University, 637371 Singapore

<sup>3</sup>Center for X-ray Optics, Lawrence Berkeley National Laboratory, Berkeley, California 94720, USA

<sup>4</sup>Department of Emerging Materials Science, DGIST, Daegu 42988, Korea

<sup>5</sup>Institute of High Performance Computing, 1 Fusionopolis Way, 138632 Singapore

### CONTENTS

---

|                                                       |    |
|-------------------------------------------------------|----|
| S1. Film Deposition and Characterization              | 2  |
| S2. Density Functional Theory Calculations            | 3  |
| S3. Hall Transport                                    | 6  |
| S4. Magnetic Interactions and Skyrmion Size Evolution | 9  |
| S5. Skyrmion Configuration Analysis                   | 11 |
| References                                            | 12 |

## S1. FILM DEPOSITION AND CHARACTERIZATION

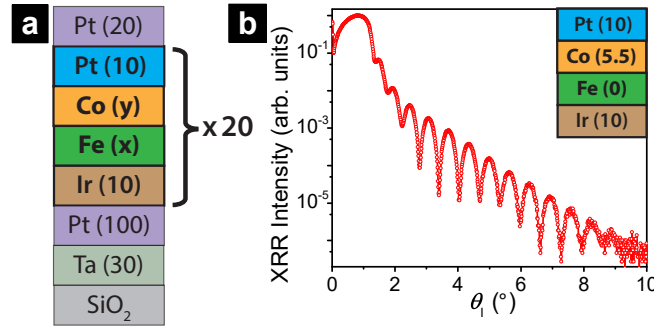

Fig. S1. **Stack Structure and Characterization.** (a) Complete stack structure of the multilayers studied in this work, with 20 repeats of Ir(10)/Fe(x)/Co(y)/Pt(10) (thickness in Å). (b) XRR measurements of the reflected intensity against incident angle ( $\theta_i$ ) for sample **Fe(0)/Co(5.5)**, with distinct Keissig fringes indicative of the sharp interfaces in the stack.

Multilayer films with [Ir(10)/Fe(x)/Co(y)/Pt(10)]<sub>20</sub> stacks (layer thickness in Å, in parentheses) were deposited on thermally oxidised 100 mm Si wafers by DC magnetron sputtering at RT, using a Chiron<sup>TM</sup> UHV system manufactured by Bestec GmbH. The base pressure before deposition was  $1 \times 10^{-8}$  Torr, and a working pressure of 1.5 mTorr of Ar gas was maintained during deposition. Seed layers of Ta (30 Å) and Pt (100 Å) were deposited before the active stacks to optimize the film texture, and a capping layer of Pt (20 Å) was added to protect the stacks against oxidation. The thickness of the Fe (0-6 Å) and Co (4-6 Å) layers were varied across the films studied in this work. The films were simultaneously deposited on Si<sub>3</sub>N<sub>4</sub> membranes (membrane thickness: 200 nm, frame size:  $5 \times 5$  mm<sup>2</sup>, window size:  $500 \times 500$  nm<sup>2</sup>, frame thickness: 200 μm, manufactured by Silson Ltd.) for MTXM measurements. The Ir/Fe/Co/Pt stacks were repeated 20 times to enhance the XMCD contrast. A schematic representation of the full multilayer stack is shown in Fig. S1a.

The deposition conditions were adjusted in order to optimize the texture, roughness, and interface quality of the multilayers. The film texture was determined from X-ray diffraction measurements, the roughness from AFM measurements, and the interface quality using X-ray reflectometry (XRR) respectively. Fig. S1b shows the XRR data obtained on a representative sample (**Fe(0)/Co(5.5)**, single stack). The persistent, oscillatory Keissig fringe pattern is indicative of the sharp nature of interfaces within the stack.

## S2. DENSITY FUNCTIONAL THEORY CALCULATIONS

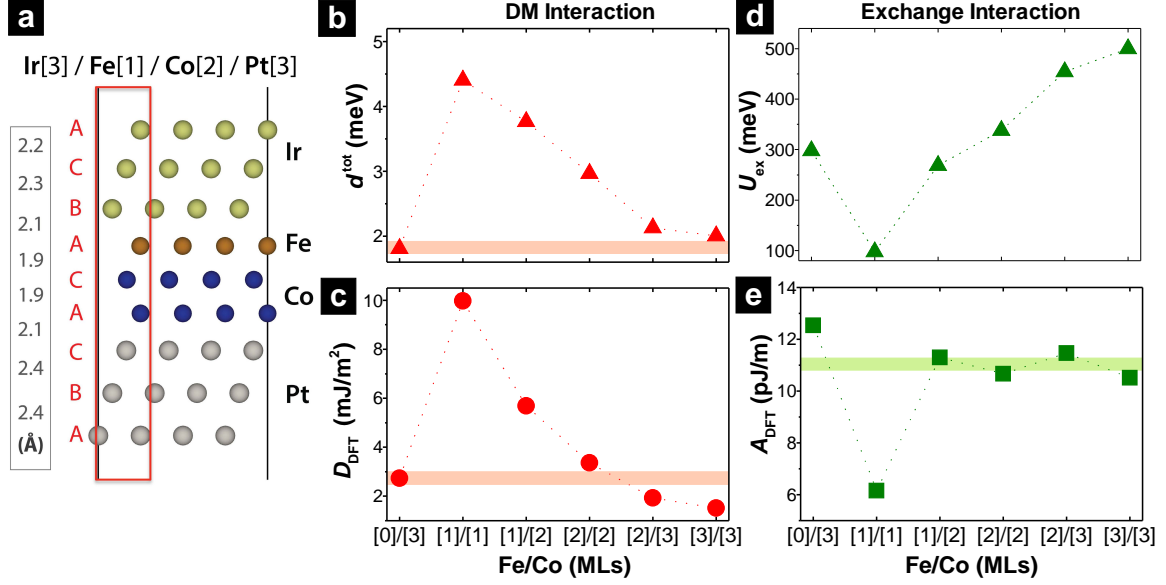

Fig. S2. **DFT Calculations of Magnetic Interactions in Ir/Fe/Co/Pt Stacks.** (a) Schematic atomic configuration of a representative multilayer stack, Ir[3]/Fe[1]/Co[2]/Pt[3], used for DFT calculations. The relaxed interlayer distances (in Å) are indicated on the left. (b-e) DFT calculated values of the DMI (b-c) and exchange interaction (d-e) for Ir[3]/Fe[a]/Co[b]/Pt[3] stacks with varying Fe/Co composition (number of atomic layers in braces). The panels show normalized atomic DMI strength,  $d^{\text{tot}}$  (b); micromagnetic DMI strength,  $D_{\text{DFT}}$  (c); exchange energy,  $U_{\text{ex}}$  (d); and exchange stiffness,  $A_{\text{DFT}}$  (e) respectively.

To compute the DMI, we performed first-principles DFT calculations at the A\*STAR Computational Resource Center, using the technique employed previously by Yang *et al.*<sup>1</sup>. The VASP package was used for the DFT calculations<sup>2</sup>. The multilayer stack, Ir[3]/Fe[a]/Co[b]/Pt[3] (number of atomic layers in braces), were set up in a close-packed configuration with (111) orientation – Pt, Fe, Ir layers were stacked in a fcc configuration while Co and adjacent layers were stacked in a hcp configuration. Each multilayer stack was separated by a vacuum of 10 Å along the OP direction, and the IP lattice constants were set to the calculated bulk Ir value, with a nearest neighbor (NN) distance of 2.74 Å. The typical atomic configuration used for the DFT calculations is shown in Fig. S2a for a representative Ir[3]/Fe[1]/Co[2]/Pt[3] stack.

### DMI Calculations

The DMI calculations were performed in three steps. First, the geometry of the system was optimized by performing structural relaxations until the forces were smaller than 0.01 eV/Å. The relaxed interlayer distances for the Ir[3]/Fe[1]/Co[2]/Pt[3] stack are indicated in Fig. S2a (left). Next, the non-spin polarized Kohn-Sham equations were solved in the absence of SOC to find an initial value for the charge density.

Subsequently, SOC and spin polarization were included and the self-consistent total energy was determined for the clockwise and counter-clockwise spin spiral configurations constructed using a constrained spin method as implemented in VASP. The Perdew-Burke-Ernzerhof (PBE) method was used for exchange correlation<sup>3</sup> and projector augmented wave (PAW) was used to represent the ionic potentials<sup>4</sup>. The Brillouin zone was sampled using a  $16 \times 4 \times 1$  Monkhorst-pack grid. Here, DMI was considered only between intralayer NN atoms to a first approximation, and used to define  $d^{\text{tot}} = \sum_k d^k$ , i.e. the sum of DMI coefficients  $d^k$  for each layer<sup>1</sup>. The energy difference between these two configurations was computed and scaled by a geometry and spin-spiral dependent factor to obtain  $d^{\text{tot}}$  (Fig. S2b), which represents the DMI strength within a single atomic layer. This was to calculate the micromagnetic DMI strength,  $D_{\text{DFT}}$  (Fig. S2c), fol-

lowing the expression<sup>1</sup>

$$D_{\text{DFT}} = \frac{3\sqrt{2}}{a^2} \cdot \frac{d^{\text{tot}}}{N_{\text{F}}} \quad (\text{S1})$$

Here,  $a$  is the fcc lattice constant and  $N_{\text{F}}$  represents the number of magnetic layers.

The effective DMI,  $D_{\text{DFT}}$  (in mJ/m<sup>2</sup>) is shown in Fig. S2c for various Fe/Co sample compositions (number of atomic layers in braces).  $D_{\text{DFT}}$  has a prominent peak for Fe[1]/Co[1], supporting the hypothesis that a stack combining Co/Pt and Fe/Ir interfaces would exhibit an additive enhancement of effective DMI.

### Exchange Interaction Calculations

We have also performed DFT calculations for the exchange stiffness  $A_{\text{DFT}}$  as it is required for quantifying skyrmion stability and other properties. To obtain  $A_{\text{DFT}}$ , we first compute an exchange energy  $U_{\text{ex}}$  (Fig. S2d) – defined as the averaged total energy of the clockwise and anti-clockwise spin spirals with respect to the total energy of the collinear spin configuration. The exchange stiffness,  $A_{\text{DFT}}$ , is then determined by equating the exchange energy density to the micromagnetic free energy as follows:

$$\frac{U_{\text{ex}}}{V_{\text{cell}}} = \frac{A_{\text{DFT}}}{2} \cdot |\nabla \vec{m}|^2 \quad (\text{S2})$$

Here  $V_{\text{cell}}$  is the unit cell volume and  $\vec{m}$  is the unit magnetization vector.

Plotted in Fig. S2e is  $A_{\text{DFT}}$  as a function of the Fe/Co layer thickness. It can be seen that  $A_{\text{DFT}}$  falls in a narrow range between 10.5 – 12.5 pJ/m for the compositions corresponding to the experimental studies. A notable exception to the trend is Fe[1]/Co[1] – with  $A_{\text{DFT}} \simeq 6.2$  pJ/m – such lowering of  $A_{\text{DFT}}$  for extremely thin magnetic multilayers has been well documented<sup>5-7</sup>.

### Anisotropy Calculations

Finally, we have also computed the magnetic anisotropy,  $K_{\text{e,DFT}}$  for Ir[3]/Fe[1]/Co[2]/Pt[3] for two stacking configurations (Fig. S3a-b), with the results detailed in Tbl. S1. The methods and details for the anisotropy calculations are similar to those for  $d^{\text{tot}}$ , with the exception that the sampling of the Brillouin zone has to be twice as dense to allow for the convergences of very small energy differences. From this calculation, we find that changing the stacking order results in a large difference in  $K_{\text{e,DFT}}$  of  $\sim 0.5$  meV. Upon dividing this difference by the magnetic volume of the system, we obtain a variation in the calculated effective anisotropy of  $\sim 2$  MJ/m<sup>3</sup> due to a change in stacking configuration – 5 times larger than the span of measured values across various sample compositions (Fig. 4d).

In fact the strong effect of stacking faults on magnetic anisotropy has been observed in previous magnetic multilayer calculations<sup>8</sup>, and one way to offset this sensitivity is to compute  $K_{\text{e,DFT}}$  averaged over numerous stacking configurations. However, this is not feasible here given the high computational cost of these calculations. Thus we have chosen to rely on the measured values of  $K_{\text{eff}}$  instead of calculated values of  $K_{\text{e,DFT}}$  in this work.

### Sensitivity of DFT Calculations

In addition, we have performed a set of DFT calculations to determine the robustness of the DFT calculated trends to structural variations. Shown in Fig. S3 are the crystal structures for the configurations of the

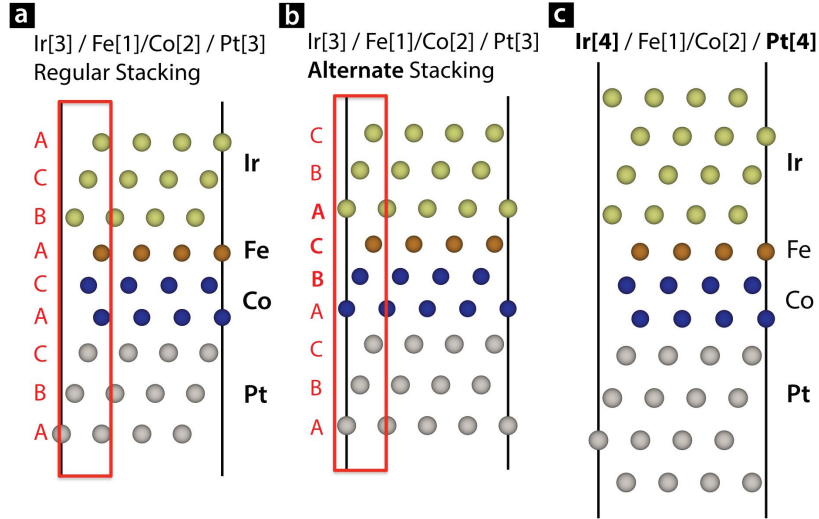

Fig. S3. **Sensitivity of DFT Calculations to Structural Variations.** Schematic atomic configurations of the Fe[1]/Co[2] multilayer stack used for investigating the sensitivity of DFT calculations to structural variations. (a) The Ir[3]/Fe[1]/Co[2]/Pt[3] stack, with close-packed configuration of layers as detailed above, used to calculate the parameters in Fig. S2d-e, serves as a control. (b) The Ir[3]/Fe[1]/Co[2]/Pt[3] stack, now containing a stacking fault, shows the sensitivity to stacking configuration. (c) The Ir[4]/Fe[1]/Co[2]/Pt[4] stack is used to study the effect of non-magnetic layer (Pt and Ir) thickness.

| Stack                               | Fig. | Exchange                   |                                | DMI                                      |                                | Anisotropy                |                                |
|-------------------------------------|------|----------------------------|--------------------------------|------------------------------------------|--------------------------------|---------------------------|--------------------------------|
|                                     |      | $A_{\text{DFT}}$<br>(pJ/m) | $\Delta A_{\text{DFT}}$<br>(%) | $D_{\text{DFT}}$<br>(mJ/m <sup>2</sup> ) | $\Delta D_{\text{DFT}}$<br>(%) | $K_{\text{DFT}}$<br>(meV) | $\Delta K_{\text{DFT}}$<br>(%) |
| Ir[3]/Fe[1]/Co[2]/Pt[3], Reg. Stack | S3a  | 11.3                       | —                              | 5.68                                     | —                              | 1.5                       | —                              |
| Ir[3]/Fe[1]/Co[2]/Pt[3], Alt. Stack | S3b  | 9.64                       | -15%                           | 6.04                                     | +6%                            | 1.0                       | -50%                           |
| Ir[4]/Fe[1]/Co[2]/Pt[4]             | S3c  | 11.5                       | +2%                            | 6.54                                     | +15%                           |                           |                                |

Table S1. **Sensitivity of DFT Calculated Magnetic Interactions to Structural Variations.** DFT calculations of exchange stiffness ( $A_{\text{DFT}}$ ), DMI strength ( $D_{\text{DFT}}$ ), and anisotropy energy ( $K_{\text{e,DFT}}$ ) for the three stack configurations shown in Fig. S3.  $A_{\text{DFT}}$  and  $D_{\text{DFT}}$  are found to be less sensitive ( $< 15\%$ ) to structural variations, while  $K_{\text{e,DFT}}$  is very sensitive to stacking order.

Fe[1]/Co[2] system used for these calculations. The system in Fig. S3a gives the  $D_{\text{DFT}}$  and  $A_{\text{DFT}}$  values for Fe[1]/Co[2] reported in Fig. S2. Using Fig. S3a as a control system, we examine the effects of varying: (1) the stacking configuration of atomic layers (Fig. S3b, with a stacking fault), and (2) the thickness of the non-magnetic (Pt and Ir) layers (Fig. S3c). The corresponding values of DMI  $D_{\text{DFT}}$ , exchange stiffness  $A_{\text{DFT}}$ , and magnetic anisotropy,  $K_{\text{e,DFT}}$  calculated for these Fe[1]/Co[2] configurations are detailed in Tbl. S1.

We find that varying the stacking order or the Pt/Ir thickness changes  $D_{\text{DFT}}$  and  $A_{\text{DFT}}$  by up to 15% from their original values. These variations in  $D_{\text{DFT}}$  and  $A_{\text{DFT}}$  are relatively small in compared to the range of range of values spanned in Fig. S2c and e respectively. Thus we do not expect the qualitative trends obtained for  $D_{\text{DFT}}$  and  $A_{\text{DFT}}$  to be affected by the stacking order and thickness of Pt and Ir layers.

In contrast, changing the stacking order results in a large change in  $K_{\text{e,DFT}}$  of  $\sim 0.5$  meV, corresponding to an effective anisotropy difference of  $\sim 2$  MJ/m<sup>3</sup>. This can in principle be offset by averaging over varying stacking configurations<sup>8</sup> for reliable anisotropy calculations, albeit at high computational costs.

### S3. HALL TRANSPORT

Electrical transport measurements were performed by defining electrical contacts (characteristic resistance  $< 0.1 \, \Omega$ ) on the films in a Hall bar configuration. The magnetoresistance and Hall coefficients were measured using a lock-in technique (excitation frequency: 0-300 Hz), enabling sub-nV resolution. The data were acquired through a full hysteresis cycle, with 2.5 mT steps within  $\pm \mu_0 H_S$  after saturation at large fields (4 T). Small AC current densities (as low as  $10^4 \, \text{A/m}^2$ ) were used for the transport measurements, so as to not perturb the spin textures. Importantly, the Hall data were analyzed after carefully accounting for any magnetic field offsets (below 0.5 mT) between magnetization and transport measurements.

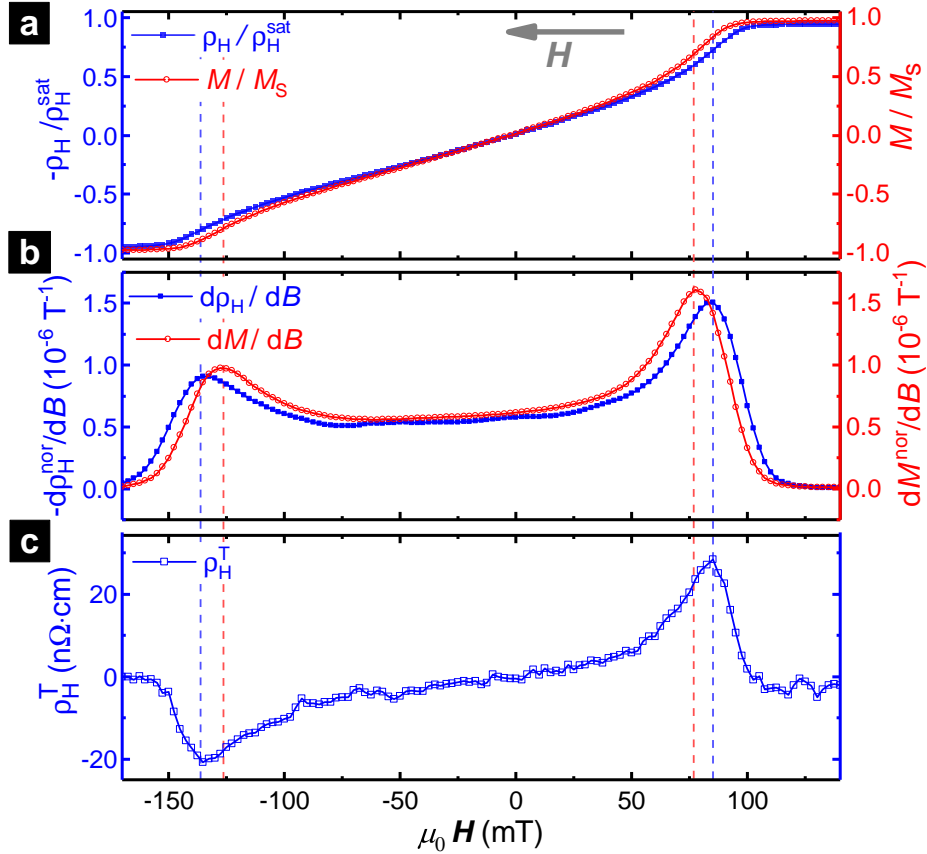

Fig. S4. **Topological Hall Effect (THE) in Fe(2)/Co(6).** (a) Normalized Hall resistivity ( $\rho_H / \rho_H^{\text{sat}}$ , blue) and OP magnetization ( $M / M_S$ , red) as a function of applied field  $B$  (grey arrow indicates sweep direction), for sample **Fe(2)/Co(6)** at RT. (b) Derivatives of  $\rho_H^{\text{nor}} \equiv \rho_H / \rho_H^{\text{sat}}$  (blue) and  $M^{\text{nor}} \equiv M / M_S$  (red) with respect to applied field  $B$ . Dashed blue and red lines indicate the peak positions of  $d\rho_H^{\text{nor}} / dB$  and  $dM^{\text{nor}} / dB$  respectively, and are offset from each other by 8-10 mT – an order of magnitude larger than any field offsets ( $< 0.5$  mT). (c) Residual Hall signal  $\rho_H^T$ , corresponding to the THE (reproduced from Fig. 3d). Note that the peaks in  $\rho_H^T$  (c, blue) are in exact correspondence with the peaks in  $d\rho_H^{\text{nor}} / dB$  (b, blue).

#### Motivation for Topological Hall Analysis

Establishing a clear distinction between the observed trends in  $\rho_H(H)$  and  $M(H)$  is useful to understand the behavior of  $\rho_H^T(H)$ . This assumes increased importance in our case due to the prominent role of magnetic anisotropy in our multilayers in comparison to previous works<sup>9-12</sup>. As a result, even a relatively large residual Hall signal (Fig. 3b,d:  $\rho_H^{T,\text{max}}$  is  $\sim 10\%$  of  $\rho_H^{\text{sat}}$ , the Hall resistivity at  $H_S$ ) appears to be relatively subtle.

To validate the THE analysis of the measured data, we carefully examine the field dependence of the

normalized Hall resistivity,  $\rho_H^{\text{nor}}(H) \equiv \rho_H / \rho_H^{\text{sat}}$  (after removing the  $H$ -linear conventional Hall term), the normalized magnetization,  $M^{\text{nor}}(H) \equiv M / M_S$ , (Fig. S4a) and their first derivatives with respect to field –  $d\rho_H^{\text{nor}}/dB$  and  $dM^{\text{nor}}/dB$  respectively (Fig. S4b). Note that the distinct peaks in  $d\rho_H^{\text{nor}}/dB$  and  $dM^{\text{nor}}/dB$  are offset from each other by 8-10 mT (blue and red dashed lines respectively), corresponding to visibly distinct inflections in the  $\rho_H(H)$  and  $M(H)$  curves respectively. These offsets in peak positions for  $d\rho_H^{\text{nor}}/dB$  and  $dM^{\text{nor}}/dB$  are an order of magnitude larger than any field offset artifacts ( $< 0.5$  mT) between the two measurements. We therefore conclude that the inflections in  $\rho_H(H)$  and  $M(H)$  occur at distinct magnetic fields.

Consequently,  $\rho_H(H)$  contains an additional unconventional anomalous contribution,  $\rho_H^{\text{T}}(H)$ , which is not proportional to  $M(H)$ . We extract  $\rho_H^{\text{T}}(H)$  by accounting for the conventional and anomalous contributions to the Hall data ( $\rho_H^{\text{T}}(H) = \rho_H(H) - \rho_H^{\text{fit}}(H)$ , see Fig. S4c). We observe that the peaks in  $\rho_H^{\text{T}}(H)$  are visibly distant from  $H_S$ , which induces sharp changes in  $\rho_H(H)$  and  $M(H)$ . Importantly, the peaks in  $\rho_H^{\text{T}}(H)$  coincide exactly with the inflections in  $\rho_H(H)$  (dashed blue lines in Fig. S4), and are visibly distinct from the corresponding features in  $M(H)$  (dashed red lines), which further justifies the analysis methodology for the Hall data.

### Robustness of Topological Hall Signal

The reproducibility of the peak magnitude and overall profile of the THE signal were verified by performing AC excitation current dependent measurements, as shown in Fig. S5a for sample Fe(2)/Co(6) over  $10^4 - 10^6$  A/m<sup>2</sup>, confirming that the spin textures that may produce the THE signal were unperturbed during the measurements.

It is also important to determine the effects of sample aging, due to the extended nature of various experiments (AFM/MFM, MTXM, magnetization, and transport) performed on these samples. In Fig. S5b, we examine the THE data acquired on sample Fe(2)/Co(6) across *three runs* spaced *over five months*. The THE peak magnitude and overall profile remain consistent across the runs. In conjunction with the consistency established across these experiments (Fig. 2-3), this suggests that aging effects on the five month time scale do not affect the observed Hall signal profile, and therefore, the magnetic interactions and skyrmion properties in these samples.

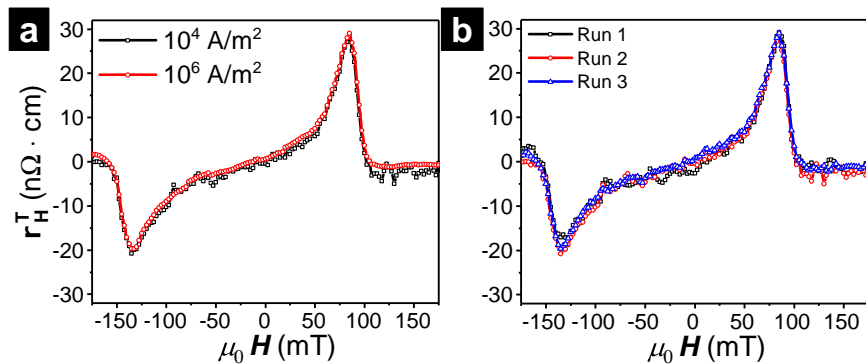

Fig. S5. **Verifying the Robustness of THE Features.** (a) AC current dependence of THE signal for sample Fe(2)/Co(6), showing no observable changes in the peak magnitude and overall profile over  $10^4 - 10^6$  A/m<sup>2</sup>. (b) Examining sample aging effects on the THE signal across three runs. Run 2 (1 month later) and Run 3 (5 months later) show no visible change, within error, compared to Run 1.

### Magnitude of Topological Hall Signal

The magnitude of  $\rho_H^T$  at RT is found to vary over  $\sim 3 - 35$  n $\Omega$ -cm across Fe/Co sample compositions, corresponding to a variation in the emergent field,  $B^T$  of 0.8–4 T within the Berry phase approximation<sup>13</sup>. Under the adiabatic (Berry phase) approximation, the measured THE signal in a skyrmion system should relate to the skyrmion density as follows:

$$\rho_H^T(H) = R_0 p_S \cdot (n_\phi^T \phi_0) \quad (\text{S3})$$

Here,  $R_0$  is the conventional ( $H$ -linear) Hall coefficient,  $p_S$  is the spin polarization of conduction electrons,  $\phi_0 \equiv h/e$  is the flux quantum, and  $n_\phi^T$  is the emergent flux density, which could correspond to the expected skyrmion density within the adiabatic approximation. In our case,  $R_0$  is determined directly from the Hall data ( $H > H_S$ , up to 4 T), and  $p_S$  ( $\equiv 0.56$ ) from previous reports on similar multilayers<sup>14</sup>. The emergent field,  $B^T = n_\phi^T \phi_0$ , relating to the THE at  $H = 0.8 H_S$ , varies over 0.8–4 T across our multilayers, corresponding to  $n_\phi^T \sim 200\text{--}900$   $\mu\text{m}^{-2}$ . Comparing this to the observed skyrmion densities in MFM images at similar fields ( $n_{\text{Sk}} \sim 6 - 60$   $\mu\text{m}^{-2}$ ), we find that the emergent flux per skyrmion,  $N_{\phi,\text{Sk}}$  varies over  $6 - 100 \phi_0$  across our multilayers.

Such a large emergent flux is in contrast to corresponding reports on Bloch materials ( $N_{\phi,\text{Sk}} \sim \mathcal{O}(1)$ <sup>9–11</sup>). A systematic field-dependent comparison between Hall transport and microscopic imaging experiments is required to address this quantitative discrepancy. Establishing a quantitative understanding of the THE and its relationship to Néel skyrmion phenomenology in such multilayers is an important next step towards its utilization for skyrmion detection in devices. The Ir/Fe/Co/Pt stack, which has now been shown to generate skyrmions with tunable properties, offers an ideal platform for such efforts.

## S4. MAGNETIC INTERACTIONS AND SKYRMION SIZE EVOLUTION

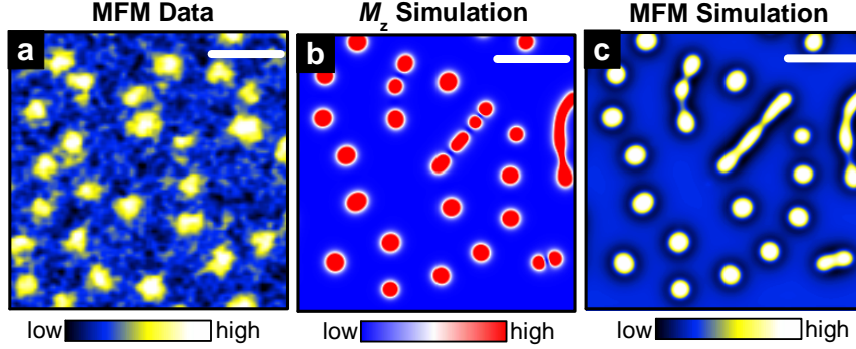

Fig. S6. **Method for Quantitative Comparison of Skyrmion Size Evolution.** Observed and simulated magnetic contrast (scale bar: 250 nm) for representative sample **Fe(4)/Co(6)** at -200 mT towards quantitative comparisons of skyrmion size evolution,  $d_{\text{Sk}}(H)$ . **(a)** Experimentally measured MFM image. **(b-c)** Simulated magnetization  $M_z$  (b), with  $D = 2.0$  mJ/m<sup>2</sup>,  $A = 14$  pJ/m (details in methods), and the corresponding simulated MFM image (c). The average skyrmion size in (c) is directly compared to that in (a), over the full field range, with varying  $D$  and  $A$  (see Fig. S7).

In our work,  $K_{\text{eff}}$  is measured directly using SQUID magnetometry. In contrast,  $D_{\text{est}}$  and  $A_{\text{est}}$  are determined indirectly, via a 2D  $\chi^2$ -fit of the MFM domain periodicity against micromagnetic simulations with varying  $D$  and  $A$ , utilizing the estimated stiffness ( $A_{\text{est}}$ ) from DFT calculations. As such, it is important to establish an independent validation of the  $A_{\text{est}}$  and  $D_{\text{est}}$  values reported in this work. In this regard, the close correspondence in Fig. 6a between the measured skyrmion size,  $d_{\text{Sk}}(H)$ , and micromagnetic simulations using ( $D_{\text{est}}$ ,  $A_{\text{est}}$ ) does support the validity of the chosen parameters. Here, we provide further evidence justifying the use of ( $D_{\text{est}}$ ,  $A_{\text{est}}$ ) obtained in Fig. 4 for modeling skyrmion behavior in these multilayers.

Micromagnetic simulations of multilayer films with numerous Fe/Co compositions were performed for direct comparison of  $d_{\text{Sk}}^{\text{MFM}}(H)$  with experiment (e.g. Fig. S6a). A randomized initial magnetization profile was allowed to relax into a stable configuration – first at zero field, and then at a series of magnetic fields (e.g. Fig. S6b) till saturation. The ‘virgin curve’ of magnetization ( $\vec{M}(x, y)$ ) images thus generated was then used to simulate corresponding MFM images (e.g. Fig. S6c) for direct comparison of  $d_{\text{Sk}}^{\text{MFM}}(H)$  with experimental data. For each of the images,  $d_{\text{Sk}}^{\text{MFM}}(H)$ , was determined by averaging over as many skyrmions (typically 5-20) as possible. The simulations were performed first using the optimal parameters ( $D_{\text{est}}$ ,  $A_{\text{est}}$ ) determined in Fig. 4e, f. Subsequently,  $D$  and  $A$  were varied around these “optimal” values to examine their validity.

A representative set of  $d_{\text{Sk}}^{\text{MFM}}(H)$  comparisons between experiments and simulations is shown in Fig. S7. Here, we examine in detail the results for sample **Fe(4)/Co(4)** ( $\kappa_{\text{est}} \simeq 1.5$ ,  $(D/A)_{\text{est}} \simeq 0.19$ ), which exhibits the smallest  $d_{\text{Sk}}^{\text{MFM}}(H)$  in our experiments. First, the results from optimal parameter ( $D_{\text{est}}$ ,  $A_{\text{est}}$ ) simulations show close correspondence with experimental data over the entire field range (Fig. S7a, red). Meanwhile, the corresponding true skyrmion size ( $d_{\text{Sk}}^{M_z}(H)$ ), determined from the simulated  $M_z$  images, shows noticeably smaller (sub-30 nm) values, justifying the claim that our MFM results ( $d_{\text{Sk}}^{\text{MFM}}(H)$ ) overestimate the true skyrmion size.

Next, we examine in Fig. S7b the effects of varying  $D$  and  $A$  by  $\sim 25\%$  around ( $D_{\text{est}}$ ,  $A_{\text{est}}$ ). For  $\kappa > 1$ , increasing  $D$  or decreasing  $A$  would lead to a faster spatial rotation of spin textures, corresponding to smaller skyrmions – consistent with the observed trends at lower fields. At higher fields, all simulated curves converge around the resolution limit ( $\sim 30$  nm) imposed by the MFM tip. Crucially, all simulated curves in Fig. S7b deviate considerably further from the measured data c.f. ( $D_{\text{est}}$ ,  $A_{\text{est}}$ ) simulations Fig. S7a.

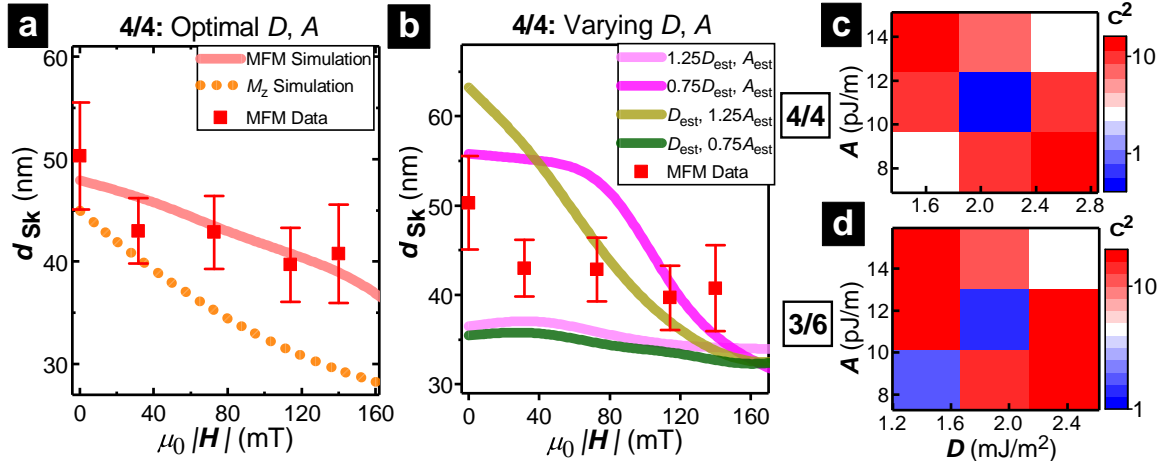

Fig. S7. **Skyrmion Size Comparison for Verification of Magnetic Parameters.** (a) Field dependence of the MFM skyrmion size,  $d_{Sk}^{MFM}(H)$ , from data acquired on sample **Fe(4)/Co(4)** (red squares), compared with micromagnetic MFM simulations (red line) using optimal ( $D$ ,  $A$ ) parameters (identified in Fig. 4e,f). The dotted orange shows the “true”  $d_{Sk}$  extracted from the associated  $M_z$  simulations. (b) Comparison of the measured  $d_{Sk}^{MFM}$  with MFM simulations, with  $D$  and  $A$  varied above and below their optimal values. The deviation from measured  $d_{Sk}^{MFM}$  is considerably higher for all curves in (b) c.f. (a). (c-d)  $\chi^2$ -fit comparison of measured and simulated  $d_{Sk}^{MFM}(H)$  for  $D$  and  $A$  varied around optimal values for representative samples **Fe(4)/Co(4)** (c) and **Fe(3)/Co(6)** (d). In both cases, the deviation from measured  $d_{Sk}^{MFM}(H)$  is demonstrably minimal for the optimal  $D, A$  simulations.

The effects of varying  $D$  and  $A$  on the goodness-of-fit of  $d_{Sk}^{MFM}(H)$  between experiments and simulations are quantified in the  $\chi^2$  plots in Fig. S7c-d for two representative samples – **Fe(4)/Co(4)** ( $\kappa_{est} \simeq 1.5$ ,  $(D/A)_{est} \simeq 0.19$ ) and **Fe(3)/Co(6)** ( $\kappa_{est} \simeq 1.1$ ,  $(D/A)_{est} \simeq 0.16$ ). In both cases, the  $(D_{est}, A_{est})$  simulations give noticeably better fits ( $\chi^2$  minima at the centre) than those from other combinations of  $D$  and  $A$ .

In summary, these  $d_{Sk}^{MFM}(H)$  results conclusively validate the magnitudes and trends of the indirectly estimated magnetic parameters ( $D_{est}, A_{est}$ ) detailed in Fig. 4e-f. The quantitative consistency of these results further demonstrates that the modulation of magnetic interactions –  $D$ ,  $K$ , and  $A$  – achieved in our multilayers by varying the Fe/Co composition, directly relates to the tuning of skyrmion properties.

## S5. SKYRMION CONFIGURATION ANALYSIS

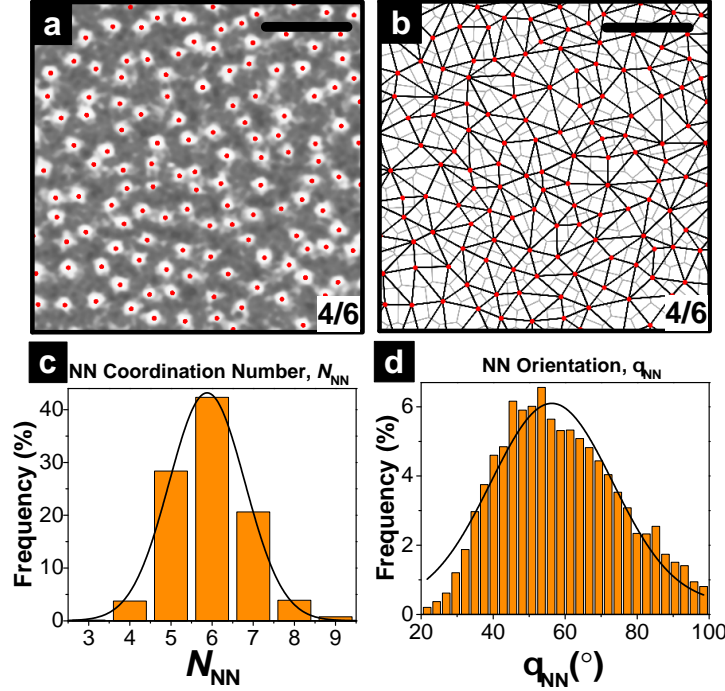

Fig. S8. **Method for Analyzing Skyrmion Configurations.** (a) MFM image (scale bar: 0.5  $\mu\text{m}$ ) of skyrmion configuration at  $H \sim -0.8 H_S$  for representative sample **Fe(4)/Co(6)**. Overlaid red dots show the centres of skyrmions identified in the image. (b) Delaunay triangulation (black lines) of the skyrmion configuration in (a), with the corresponding Voronoi cells in light grey. Nearest neighbor (NN) statistics generated from the triangulation method: (c) NN coordination number,  $N_{NN}$ , and (d) NN angular orientation,  $\theta_{NN}$ , with overlaid black lines showing Gaussian fits.

In order to quantify the influence of thermodynamic stability,  $\kappa$ , we analyze the skyrmion configurations in MFM images acquired at  $H \sim -0.8 H_S$ , close to the maximal observed skyrmion density across samples. To this end, we use the Delaunay triangulation method (Fig. S8), which has been extensively used for analyzing configurations of superconducting vortices (see e.g. Song *et al.*<sup>15</sup>).

We begin by determining the centre positions of skyrmions in the image. The skyrmions are identified by binarized thresholding of the image, and are fitted using a 2D isotropic Gaussian function to determine the centres. The red dots overlaid in Fig. S8a show the skyrmion centres identified using this technique.

Delaunay triangulation, when performed on a set of points, ensures that no point is inside the circum-circle of any triangle in the image. The result of this triangulation, performed on the skyrmion centres, is shown in Fig. S8b. This can be used to determine the nearest neighbour (NN) statistics, and thereby quantify the order in skyrmion configurations. We evaluate histograms of: (a) NN coordination number,  $N_{NN}$  (the number of lines connected to each red dot, Fig. S8c), and (b) NN angular orientation,  $\theta_{NN}$  (the angle between neighboring lines connected to each dot, Fig. S8d).

For an ideal hexagonal lattice,  $N_{NN} = 6$  and  $\theta_{NN} = 60^\circ$ . The histograms for **Fe(4)/Co(6)** (Fig. S8c-d), while centered at these values, have an observable spread. This corresponds to a short-range hexagonally ordered, or glassy phase, which we refer to as a disordered lattice. For  $\kappa_{\text{est}} < 1$ , the distributions correspond to isolated skyrmions (Fig. 5 bottom), deviating considerably from ( $N_{NN} = 6$ ,  $\theta_{NN} = 60^\circ$ ), and with a larger spread. With increasing  $\kappa_{\text{est}}$ , the distributions gradually converge around these values, indicating a disordered hexagonal skyrmion lattice (Fig. 5 top).

---

\* [souma@dsi.a-star.edu.sg](mailto:souma@dsi.a-star.edu.sg)

† [christos@ntu.edu.sg](mailto:christos@ntu.edu.sg)

- [1] Yang, H., Thiaville, A., Rohart, S., Fert, A. & Chshiev, M. Anatomy of Dzyaloshinskii-Moriya Interaction at Co/Pt Interfaces. *Physical Review Letters* **115**, 267210 (2015).
- [2] Kresse, G. & Furthmüller, J. Efficiency of ab-initio total energy calculations for metals and semiconductors using a plane-wave basis set. *Computational Materials Science* **6**, 15–50 (1996).
- [3] Perdew, J. P., Burke, K. & Ernzerhof, M. Generalized Gradient Approximation Made Simple. *Physical Review Letters* **77**, 3865–3868 (1996).
- [4] Kresse, G. & Joubert, D. From ultrasoft pseudopotentials to the projector augmented-wave method. *Physical Review B* **59**, 1758–1775 (1999).
- [5] Heinze, S. *et al.* Spontaneous atomic-scale magnetic skyrmion lattice in two dimensions. *Nature Physics* **7**, 713–718 (2011).
- [6] Dupé, B., Hoffmann, M., Paillard, C. & Heinze, S. Tailoring magnetic skyrmions in ultra-thin transition metal films. *Nature Communications* **5**, 4030 (2014).
- [7] Dupé, B., Bihlmayer, G., Böttcher, M., Blügel, S. & Heinze, S. Engineering skyrmions in transition-metal multilayers for spintronics. *Nature Communications* **7**, 11779 (2016).
- [8] Wu, G. *et al.* First-principles calculations of the magnetic anisotropic constants of Co-Pd multilayers: Effect of stacking faults. *Europhysics Letters* **99**, 17001 (2012).
- [9] Neubauer, A. *et al.* Topological Hall Effect in the A Phase of MnSi. *Physical Review Letters* **102**, 186602 (2009).
- [10] Huang, S. X. & Chien, C. L. Extended Skyrmion Phase in Epitaxial FeGe(111) Thin Films. *Physical Review Letters* **108**, 267201 (2012).
- [11] Porter, N. A., Gartside, J. C. & Marrows, C. H. Scattering mechanisms in textured FeGe thin films: Magnetoresistance and the anomalous Hall effect. *Physical Review B* **90**, 024403 (2014).
- [12] Matsuno, J. *et al.* Interface-driven topological Hall effect in SrRuO<sub>3</sub>-SrIrO<sub>3</sub> bilayer. *Science Advances* **2**, e1600304 (2016).
- [13] Nagaosa, N. & Tokura, Y. Topological properties and dynamics of magnetic skyrmions. *Nature Nanotechnology* **8**, 899–911 (2013).
- [14] Rajanikanth, A., Kasai, S., Ohshima, N. & Hono, K. Spin polarization of currents in Co/Pt multilayer and Co-Pt alloy thin films. *Applied Physics Letters* **97**, 022505 (2010).
- [15] Song, C.-L. *et al.* Dopant clustering, electronic inhomogeneity, and vortex pinning in iron-based superconductors. *Physical Review B* **87**, 214519 (2013).
